# Supplementary material for: The homotopy type of the cobordism category
Source: arXiv:math/0605249 source file (2010-09-21)
Supplement: Supplementary file 1 [file appendix.tex]

\appendix

\section{Segal's category}
\label{sec:segals-category}

Segal's category $\mathcal{S}$ of conformal surfaces is similar to our
cobordism category $\mathcal{C}_2^+$ of oriented surfaces.  The main
difference is that in his category, a morphism is an isomorphism class
of Riemann surfaces with parametrized boundary, and in ours it is an
oriented surface in $\setR^\infty$.  We give a precise definition of
$\mathcal{S}$ in \ref{defn:S} below.  There is also a ``positive
boundary'' version $\mathcal{S}_\partial$.  The main result of this
appendix is the following theorem.
\begin{theorem}\label{thm:Segals-cat}
  There is a rational isomorphism
  \begin{align*}
    B\mathcal{S} \simeq_{\setQ} B\mathcal{C}_2^+
  \end{align*}
  and a homotopy equivalence of positive boundary categories
  \begin{align*}
    B\mathcal{S}_\partial \simeq B\mathcal{C}_{2,\partial}^+.
  \end{align*}
\end{theorem}

% We give a precise definition of Segal's version $\mathcal{S}$ of the
% 2-dimensional cobordism category and prove that its classifying space
% $B\mathcal{S}$ is rationally equivalent to $B\mathcal{C}_2^+$.  
Morphism spaces in Segal's category are moduli spaces of Riemann
surfaces with parametrized boundary.  The connected components of
these moduli spaces are labelled by the topological type of the
underlying oriented 2-manifold.  More precisely, suppose $\Sigma$ is
an oriented 2-manifold with collared boundary.  The collar gives a
complex structure on $\Sigma$ near the boundary, and we let
$J(\Sigma)$ be the space of complex structures on $\Sigma$ which agree
with the fixed one near the boundary.  Let $\Diff^+(\Sigma,\partial
\Sigma)$ be the group of oriented diffeomorphisms of $\Sigma$ which
restrict to the identity near the boundary, and let
$\mathcal{M}_\Sigma$ be the quotient space
\begin{align*}
  \mathcal{M}_\Sigma = J(\Sigma)/\Diff^+(\Sigma,\partial \Sigma).
\end{align*}
If $\Sigma$ is a closed, connected surface of genus $g$ we have a
homeomorphism to Riemann's moduli space $\mathcal{M}_g$.
% Let us also point out that $\mathcal{M}_\Sigma$ is infinite
% dimensional if $\partial \Sigma \neq \emptyset$.  Indeed, it has a
% free action of $\Diff(S^1)$ by reparametrizing a boundary component.

The product $E\Diff^+(\Sigma,\partial \Sigma) \times J(\Sigma)$ has a
free action of $\Diff(\Sigma)$ and we get two projection maps from the
quotient
\begin{align*}
  B\Diff^+(\Sigma,\partial \Sigma) \leftarrow
  (E\Diff^+(\Sigma,\partial \Sigma) \times
  J(\Sigma))/\Diff^+(\Sigma,\partial \Sigma) \rightarrow
  \mathcal{M}_\Sigma.
\end{align*}
The projection onto $B\Diff^+(\Sigma,\partial \Sigma)$ is a fiber
bundle with fiber $J(\Sigma)$ and hence a homotopy equivalence.
Therefore we get a map
\begin{align}
  \label{eq:31}
  B\Diff^+(\Sigma, \partial \Sigma) \to \mathcal{M}_\Sigma,
\end{align}
well defined up to homotopy.  Roughly speaking, the quotient
map~\eqref{eq:31} gives rise to a map $B\mathcal{C}_2^+ \to
B\mathcal{S}$ (actually there is a zig-zag of functors, cf.\
diagram~\eqref{eq:30} below, but the step related to~\eqref{eq:31} is
the most important one).  In the case where all connected components
of $\Sigma$ have non-empty boundary, for example if $\Sigma$ satisfies
the positive boundary condition, the action of
$\Diff^+(\Sigma,\partial \Sigma)$ on $J(\Sigma)$ is free, and the
map~\eqref{eq:31} is a homotopy equivalence.  In the case where all
closed connected components have genus at least 2, the action has
finite isotropy groups (this is Schwarz's theorem (\cite{SCHWARZ}),
see also e.g.\ \cite[chapter V]{MR583745}), and hence~\eqref{eq:31} is
a rational equivalence.  The main challenge in proving
$B\mathcal{C}_2^+ \simeq_\setQ B\mathcal{S}$ is to deal with the
remaining case in which $\Sigma$ has components which are spheres or
tori.

%   It is a standard fact that the
% automorphism group of a Riemann surface $\Sigma$ is finite, except for
% the two exceptional cases where $\Sigma$ is diffeomorphic to a sphere
% or to a torus.  In all other cases the quotient map
% \begin{align*}
%   B\Diff^+(\Sigma,\partial \Sigma) \to \mathcal{M}_\Sigma
% \end{align*}
% is a rational equivalence.  The main challenge in proving
% $B\mathcal{C}_2^+ \simeq_\setQ B\mathcal{S}$ is to deal with spheres
% and tori.

We proceed to give a definition of Segal's category $\mathcal{S}$.
The proof of $B\mathcal{C}_2^+\simeq_\setQ B\mathcal{S}$ will consist
of a zig-zag of weak equivalences, and we also define the spaces
involved in this zig-zag.  All the spaces are classifying spaces of
categories.  The proof is organized according to the following diagram
of categories and functors.
\begin{align}\label{eq:30}
  \begin{aligned}
    \xymatrix{
      & \mathcal{C}_\partial \ar[d] &  \mathcal{C}^p_\partial
      \ar[d]\ar[l] & \mathcal{S} \ar[d]\\
      \mathcal{C}_2^+ \ar[r] & \mathcal{C} & \mathcal{C}^p
      \ar[l]\ar[r] & \overline{\mathcal{C}}
    }
  \end{aligned}
\end{align}
The category $\mathcal{C}$ is the ``reduced'' version of
$\mathcal{C}_2^+$ from Remark~\ref{rem:1}.  Thus, the leftmost
horizontal functor induces a weak equivalence $B\mathcal{C}_2^+ \to
B\mathcal{C}$.  The two categories with subscript $\partial$ in the
top row are ``positive boundary'' versions of the categories below
them in the diagram.  Going from the second to the third column we
change the space of objects: In the second column an object is an
``unparametrized'' 1-manifold $S \subseteq \setR^{1+\infty}$, in the
third we include a parametrization $\phi: \{1, \dots, n\} \times S^1
\to S$ in the data of an object.  Going from the third to the fourth
we replace $B\Diff(\Sigma,\partial \Sigma)$ by $\mathcal{M}_\Sigma$;
this is the main step of the proof.

\begin{definition}
  Let $\mathcal{C}^p$ be the category whose objects are pairs $(S,p)$,
  where $S$ is an object of $\mathcal{C}$ (i.e.\ $S\subseteq
  \setR^{d-1+\infty}$ is a closed oriented 1-manifold), and $p$ is a
  diffeomorphism
  \begin{align*}
    p: \{1,\dots, n\} \times S^1 \to S.
  \end{align*}
  The morphisms from $(S_0,p_0)$ to $(S_1, p_1)$ are pairs $(W,a,j)$,
  where $(W,a) \in \mathcal{C}_2(S_0, S_1)$ (i.e.\ $W \subseteq [0,a]
  \times \setR^{d-1+\infty}$ is an cobordism), and $j$ is a complex
  structure on $W$ compatible with the orientation.  The collars of
  $W$ give unique extensions
  \begin{align*}
    p_{\mathrm{in}}: \{1, \dots, n_{\mathrm{in}}\} \times S^1 \times
    [0,\epsilon) &\to W\\
    p_{\mathrm{out}}: \{1, \dots, n_{\mathrm{out}}\} \times S^1 \times
    (-\epsilon,0] &\to W
  \end{align*}
  and we require these to be holomorphic for small $\epsilon$ (this
  fixes $j$ near the boundary).
\end{definition}
\begin{definition}
  Let $\overline{\mathcal{C}}$ be the category with the same space
  of objects as $\mathcal{C}^p$ and morphisms
  \begin{align*}
    \overline{\mathcal{C}}((S_0, p_0),(S_1, p_1)) =
    \mathcal{C}^p(S_0, S_1)/\sim,
  \end{align*}
  where $\sim$ denotes biholomorphic equivalence: $(W,a,j) \sim
  (W',a',j')$ if there is a diffeomorphism $\phi: W \to W'$, fixing a
  neighborhood of the boundary, which is holomorphic with respect to
  $j$ and $j'$.
\end{definition}
\begin{definition}\label{defn:S}
  For each $n \in \setN$, pick an embedding
  \begin{align*}
    \phi_n: \{1, \dots, n\} \times S^1 \to \setR^2 \subseteq
    \setR^{d-1+\infty}.
  \end{align*}
  This defines an object $C_n \in \overline{\mathcal{C}}$, and we
  let $\mathcal{S}$ be the full subcategory of
  $\overline{\mathcal{C}}$ with these objects.
\end{definition}
$\mathcal{S}$ is our interpretation of Segal's category.  It has
objects $\setN$, and morphisms $\mathcal{S}(n,m)$ is the disjoint
union
\begin{align*}
  \mathcal{S}(n,m) =\coprod_\Sigma \mathcal{M}_\Sigma,
\end{align*}
where $\Sigma$ runs over cobordisms from $n$ circles to $m$ circles,
one in each diffeomorphism class.  The positive boundary version
$\mathcal{S}_\partial$ is defined by taking only disjoint union over
cobordisms in which each component has at least one outgoing boundary
circle.

We have functors $\mathcal{S} \rightarrow \overline{\mathcal{C}}
\leftarrow \mathcal{C}^p \rightarrow \mathcal{C}$.
\begin{lemma}\label{lem:S-Cbar}
  The inclusion $\mathcal{S} \to \overline{\mathcal{C}}$ induces a
  weak equivalence $B\mathcal{S} \to B\overline{\mathcal{C}}$.
\end{lemma}
\begin{proof}
  For each $k$, the inclusion
  \begin{align*}
    N_k \mathcal{S} \to N_k\overline{\mathcal{C}}
  \end{align*}
  is a weak equivalence, because the space of embeddings $\{1, \dots,
  n\} \times S^1 \to \setR^{d-1+\infty}$ is contractible.
\end{proof}
\begin{lemma}\label{lem:forget-param}
  The functor $\mathcal{C}^p \to \mathcal{C}$, which forgets the
  parametrizations of objects and the complex structure on morphisms,
  induces a weak equivalence $B\mathcal{C}^p \to B\mathcal{C}$.
\end{lemma}
\begin{proof}
  For a given orientation on a morphism $W$, the space of compatible
  complex structures is contractible, so forgetting the complex
  structure does not change homotopy types.

  The space of parametrizations of a 1-manifold is not contractible,
  but we can use essentially the same proof as given in
  Section~\ref{sec:proof-of-main-theorem} of the equivalence
  $B\mathcal{C} \simeq |D_2|$ to prove that $B\mathcal{C}^p \simeq
  |D_2|$.  All the sheaves $D_2^\pitchfork$, $C_2^\perp$ and
  $C_2^\pitchfork$ used in that proof have enriched versions where all
  circles are parametrized by some standard circle $S^1$.  The main
  point of the proof is then in Proposition~\ref{prop:5}: If we choose
  the open sets $U_j$ contractible, the bundles $(f_j)^{-1}(a_j) \to
  U_j$ will be trivializable.  Arrange that all regular values $a_j$
  are different, and choose parametrizations
  \begin{align}
    \phi_j : U_j \times (\{1, \dots, n_j\} \times S^1) \to
    (f_j)^{-1}(a_j).\tag*{\qedhere}
  \end{align}
\end{proof}

It remains to prove that $B\mathcal{C}^p \to B\overline{\mathcal{C}}$
is a rational equivalence.  To this end we consider two more spaces
\begin{definition}
  Let $\mathcal{C}^p_\partial \subseteq \mathcal{C}^p$ be the
  subcategory with the same objects, but where morphisms are required
  to be ``positive boundary'' (i.e.\ all connected components of a
  cobordism have non-empty outgoing boundary).
\end{definition}
\begin{lemma}\label{lem:connect-param}
  The inclusion $B\mathcal{C}^p_\partial \to B\mathcal{C}^p$ is a weak
  equivalence.
\end{lemma}
\begin{proof}
  In the same way as in Lemma~\ref{lem:forget-param}, we prove that
  $B\mathcal{C}^p_\partial \to B\mathcal{C}_\partial\simeq
  B\mathcal{C}_{2,\partial}^+$ is a weak equivalence.  Then the result
  follows from Theorem~\ref{thm:connectedness}.
\end{proof}

Finally we need a modified version of $B\mathcal{C}^p$.  A
non-identity morphism in $\mathcal{C}^p$ is given by a real number $a
> 0$, a cobordism $W \subseteq [0, a] \times \setR^{d-1+\infty}$, and
parametrizations of $\partial W$.  We will focus on connected
components of $W$ which are diffeomorphic to either a sphere $S^2$ or
a torus $T^2 = S^1 \times S^1$.  Let us say that a connected component
$C \subseteq W$ is \emph{tame} if it is not diffeomorphic to one of
these.  If $C$ is diffeomorphic to $T^2$, let us say that a
\emph{taming} is a choice of a point $p \in C$, and if $C$ is
diffeomorphic to $S^2$, a taming is a choice of a non-zero tangent
vector $v \in TC$.  A \emph{taming} of a morphism is a choice of one
(and only one) taming of each non-tame connected components.  We now
consider a version of $N_\bullet \mathcal{C}^p$, where all morphisms
are equipped with tamings.
\begin{definition}\label{def:Xk}
  For $k \geq 0$, let $X_k$ be the set of pairs $(\chi,T)$, where
  $\chi \in N_k \mathcal{C}^p$ is a non-degenerate simplex, i.e.\ a
  tuple $\chi = (f_1, \dots, f_k)$ of composable non-identity
  morphisms in $\mathcal{C}^p$, together with a $k$-tuple $T = (t_1,
  \dots, t_k)$ where each $t_i$ is a taming of the manifold $W_i$
  underlying the morphism $f_i$.
\end{definition}
Let $N^{\mathrm{nd}}_k \mathcal{C}^p$ denote the space of
non-degenerate $k$-simplices.  Then there is a map $X_k \to
N^{\mathrm{nd}}_k \mathcal{C}^p$ which forgets the tamings.
\begin{lemma}\label{lem:X-overlineC}
  For each $k$, the composition
  \begin{align}\label{eq:37}
    X_k \to N^{\mathrm{nd}}_k \mathcal{C}^p \to N_k^{\mathrm{nd}}
    \overline{C}
  \end{align}
  is a rational equivalence.
\end{lemma}
\begin{proof}
  Let us first consider $k=1$.  Then on each connected component, the
  composition~\eqref{eq:37} is of the form
  \begin{align*}
    B\Diff^+(\Sigma,t \cup \partial \Sigma) \to
    B\Diff^+(\Sigma,\partial \Sigma) \to \mathcal{M}_\Sigma.
  \end{align*}
  Here, $t$ is a taming of $\Sigma$, possibly empty (if $\Sigma$ is
  already tame), and $\Diff^+(\Sigma,t \cup \partial \Sigma)$ is the
  group of diffeomorphisms of $\Sigma$ which fixes the taming and acts
  as the identity on the boundary.  This map is better behaved
  than~\eqref{eq:31} above in that the stabilizers of the actions of
  $\Diff^+(\Sigma,t \cup \partial \Sigma)$ on $J(\Sigma)$ has trivial
  rational homology for \emph{all} surfaces $\Sigma$.  To see this, we
  need only consider the two special cases $S^2$ and $T^2$.  Any
  complex structure on $S^2$ is holomorphically equivalent to the
  Riemann sphere $\mathbbm{P}^1$ which has automorphism group
  $P\mathrm{Sl}_2(\setC)$.  We can assume that the taming is given by
  the tangent vector $\partial/\partial z$ at the point $0 \in
  \mathbbm{P}^1$.  The diffeomorphisms which preserve the complex
  structure and this framing is the group of M\"obius transformations
  of the form $z \mapsto z/(1+cz)$ for $c \in \setC$.  This group is
  isomorphic to the topological group $(\setC, +)$ and hence has
  contractible classifying space.  The case $T^2$ follows from
  (elementary) theory of elliptic curves: for any complex structure on
  $T^2$, it is isomorphic to $\setC/\Lambda$ for some lattice
  $\Lambda\subseteq \setC$.  We can assume that the taming is given by
  the point $0 +\Lambda$.  The diffeomorphisms which preserves the
  taming and the complex structures are now the automorphisms of the
  elliptic curve; depending on $\Lambda$, the group of such is either
  $\setZ/2$, $\setZ/4$, or $\setZ/6$, and hence has rationally trivial
  classifying space.

  This finishes the case $k=1$.  Higher values of $k$ are obtained by
  taking products of the case $k=1$.
\end{proof}

Unfortunately, the spaces $X_k$ do not form a simplicial space
(degeneracies not well defined).  However they do form a poset whose
classifying space maps to $B\mathcal{C}^p$, via the simplicial
subdivision of $N_\bullet\mathcal{C}^p$.  We recall some definitions.
The spaces $N_k^{\mathrm{nd}}\mathcal{C}^p$ can be united to a
topological poset
\begin{align*}
  PN_\bullet\mathcal{C}^p = \coprod_k N_k^{\mathrm{nd}}\mathcal{C}^p,
\end{align*}
ordered by inclusion: If $\chi \in N_k^{\mathrm{nd}}\mathcal{C}^p$ and
$\chi' \in N_l^{\mathrm{nd}}\mathcal{C}^p$, then $\chi < \chi'$ if
there is a map $\theta \in \Delta(k,l)$ such that $\theta^*(\chi') =
\chi$.  The nerve of $PN_k\mathcal{C}^p$ is the simplicial subdivision
of the nerve of $\mathcal{C}^p$, and they have homeomorphic
realizations
\begin{align*}
  B(PN_\bullet\mathcal{C}^p) \cong B\mathcal{C}^p.
\end{align*}
Similarly we have a poset $PN_k\overline{\mathcal{C}}$ of
non-degenerate simplices of $N_k\overline{\mathcal{C}}$ and a
homeomorphism
\begin{align*}
  B(PN_\bullet\overline{\mathcal{C}}) \cong B\overline{\mathcal{C}}.
\end{align*}
Finally, the spaces $X_k$ unite to a topological poset
\begin{align*}
  X = \coprod_k X_k,
\end{align*}
where the ordering is $(\chi, T) < (\chi', T')$ if $\chi < \chi'$ and
$\cup t_i \supseteq \cup t_i'$.  This is well defined and there are
map of posets
\begin{align}\label{eq:41}
  X \to PN_\bullet\mathcal{C}^p \to PN_\bullet\overline{\mathcal{C}},
\end{align}
where the first map is the one that forgets tamings.  We have the
following lemma.
\begin{lemma}\label{lem:rational-eq}
  The composition
  \begin{align*}
    BX \to B\mathcal{C}^p \to B\overline{\mathcal{C}}
  \end{align*}
  induced by~\eqref{eq:41}, is a rational equivalence.
\end{lemma}
\begin{proof}
  Consider the map
  \begin{align*}
    N_k X \to N_kPN_\bullet\mathcal{C}^p \to
    N_kPN_\bullet\overline{\mathcal{C}}.
  \end{align*}
  For $k =0$ this is the same map as~\eqref{eq:37} and hence a
  rational equivalence.  The case $k > 0$ is similar, and hence the
  induced map on geometric realization is a rational equivalence.  \textbf{[FIXME]}
\end{proof}

\begin{corollary}\label{cor:Cp-Cbar}
  The quotient map $B\mathcal{C}^p \to B\overline{\mathcal{C}}$ is a
  rational equivalence.
\end{corollary}
\begin{proof}
  Notice that the inclusion $B\mathcal{C}^p_\partial \to
  B\mathcal{C}^p$ factors through $BX_\bullet$.  Consider the
  composition
  \begin{align*}
    B\mathcal{C}^p_\partial \to \|X_\bullet\| \to B\mathcal{C}^p \to
    B\overline{\mathcal{C}}.
  \end{align*}
  The composition of the first two maps is a weak equivalence by
  Lemma~\ref{lem:connect-param}, and the composition of the last two
  maps is a rational equivalence by Lemma~\ref{lem:rational-eq}.
\end{proof}
\begin{proof}[Proof of theorem~\ref{sec:segals-category}]
  The first part of the theorem follows by combining
  lemma~\ref{lem:S-Cbar} with lemma~\ref{cor:Cp-Cbar}.

  For the second part of the statement, let
  $\overline{\mathcal{C}}_\partial$ denote the positive boundary
  version of $\overline{\mathcal{C}}$, defined in the obvious way.
  Then we have the following positive boundary version of
  diagram~\eqref{eq:30}.
  \begin{align}\label{eq:34}
    \mathcal{S}_\partial \rightarrow \overline{\mathcal{C}}_\partial
    \leftarrow \mathcal{C}_\partial^p \rightarrow \mathcal{C}_\partial,
  \end{align}
  and a similar diagram after applying $B$.  This diagram is similar
  to~\eqref{eq:30}, only easier: On morphism spaces, the middle arrow
  $\mathcal{C}_\partial^p \to \overline{\mathcal{C}}_\partial$ is of
  the form~\eqref{eq:31}, but involves only surfaces $\Sigma$ without
  closed components.  Hence 
  \begin{align*}
    N_k\mathcal{C}_\partial^p \to N_k\overline{\mathcal{C}}_\partial
  \end{align*}
  is a homotopy equivalence for all $k$.  The outer arrows
  in~\eqref{eq:34} are treated exactly as the corresponding arrows
  in~\eqref{eq:30}.
\end{proof}

%%% Local Variables: 
%%% mode: latex
%%% TeX-master: "GMTW"
%%% End: 
